# Supplementary material for: HeterMoE: Efficient Training of Mixture-of-Experts Models on Heterogeneous GPUs
Source: arXiv:2504.03871 source file (2025-04-04)
Supplement: Supplementary file 1 [file appendix.tex]

\appendix
\section{Appendix}

\subsection{Proof of~\autoref{algo:asymea}}
To prove that optimal balancing can be achieved by~\autoref{algo:asymea} as long as there are many micro-batches, we need to show that GPU attention is always busy. Since we cannot control the communication time, the best thing \asymabbr can do is to make sure the expert GPU is not delaying the starting time of successor layer's attention computation during gathering phase by satisfying the following condition,
\begin{align}
    L\cdot m T^{\attngpusym}_A \geq T^{\attngpusym}_A + T^{\expgpusym}_E+  (L-1)\cdot mT^{\expgpusym}_E,
\end{align}
where $L$ is the number of \textbf{finished} layers and $L>0$ since the first layer's attention has no dependency on expert GPU, and $m$ is the number of micro-batches in \parallelism. We assume that for the previous $L$ layers and $m$ micro-batches, both attention and expert GPUs are busy. 

We will prove that this condition holds before we reach the next expert offloading point. The above relation can be reordered as,
\begin{align}
    (L\cdot m - 1) T^{\attngpusym}_A &\geq (L-1)\cdot mT^{\expgpusym}_E + T^{\expgpusym}_E \\
    \frac{T^{\attngpusym}_A}{T^{\expgpusym}_E} &\geq \frac{(L-1)\cdot m + 1}{(L\cdot m - 1) } \\
    \frac{T^{\attngpusym}_A}{T^{\expgpusym}_E} &\geq \frac{L-1 + \frac{1}{m}}{(L - \frac{1}{m}) }.
\end{align}
Suppose the $m$ is very large, the relation can be simplified as,
\begin{align}
    \frac{T^{\attngpusym}_A}{T^{\expgpusym}_E} &\geq \frac{L-1}{L} \\
    L &\leq \frac{T^{\expgpusym}_E}{T^{\expgpusym}_E - T^{\attngpusym}_A} \\
    L_{\text{busy}} &= \frac{T^{\expgpusym}_E}{T^{\expgpusym}_E - T^{\attngpusym}_A}
\end{align}
which means without any expert offloading, the expert GPUs won't delay the beginning of successor attention until the attention GPU finishes $L_{\text{busy}}$ layers. Note that $T_{\text{gather}} =  T^{\expgpusym}_{E}-T^{\attngpusym}_{A}$, so the accumulated bubble at this time will be
\begin{align}
    t_{bubble} = L_{\text{busy}} \cdot T_{\text{gather}} = T^{\expgpusym}_E \geq T_{\text{squeeze}},
\end{align}
which means a "squeeze" has to happen before or right at this layer. After this layer the lagging on the expert GPU is reset and the following layers can be proved in the same way. 
In practice, although there is communication delay and the number of micro-batches can be limited, an expert GPU usually employs multiple experts, so it won't wait until $L_{\text{busy}}$ to offload experts and the overall bubbles will be minimized.

\subsection{Benefits of ~\autoref{algo:asymea} on AWS} 

See Figure~\autoref{fig:ablation_asymea_aws}.

\begin{figure}
    \begin{subfigure}{0.48\linewidth}
        \centering
        \includegraphics[width=\linewidth]{figures/asymea/asymea_greatlakes_Mixtral-D1_C1.pdf}
        \caption{Mixtral-C1 on D1 \xueshen{up to 1.65x}}
        \label{fig:ablation_asymea_d1_c1}
    \end{subfigure} \hfil
    \begin{subfigure}{0.48\linewidth}
        \centering
          \includegraphics[width=\linewidth]{figures/asymea/asymea_greatlakes_Mixtral-D3_C2.pdf}
        \caption{Mixtral-C2 on D3 \xueshen{upto 1.42x}}
        \label{fig:ablation_asymea_d1_c2}
    \end{subfigure}
\caption{\textbf{[Ablation Study]:} Speed-up provided by \sys's \asymabbr in terms of training throughput, compared to \sys without \asymabbr.}
\label{fig:ablation_asymea_aws}
\end{figure}

\subsection{Theoretical Speed-up of \sys}
To validate our results, we calculate the theoretical speedup \sys is supposed to achieve. According to \autoref{fig:background_speedup_a40_v100}, when processing a sequence with 20k tokens, A40 is about 1.18x faster than V100 on expert while about 3x faster on attention. Our profiler shows that $T^{A}_{\attngpusym} = 1.05\cdot T^{E}_{\expgpusym}$. To simplify the calculation, let us make the following approximation of computation time per sequence,
\begin{align}
    T^{A}_{\attngpusym} &= T^{E}_{\expgpusym} = T^{E}_{\expgpusym} = t \\
    T^{E}_{\attngpusym} &= 3\cdot T^{A}_{\attngpusym} = 3t 
\end{align}
Assume the model has $L$ layers.
EP~(Ideal) runs A40 and V100 separately, so the total throughput $P_{EP~(Ideal)}$ is calculated as 
\begin{align}
    P_{EP~(Ideal)} = \frac{1}{(T^{A}_{\attngpusym}+T^{E}_{\attngpusym})\cdot L} + \frac{1}{(T^{A}_{\expgpusym}+T^{E}_{\expgpusym})\cdot L} = \frac{3}{4Lt}.
\end{align}
While in \sys, every transformer layers is decoupled into two stages, i.e. attention and expert. Therefore, the time to process $2n$ samples is 
\begin{align}
    T_{\sys} &= T^{A}_{\attngpusym} + n\cdot (T^{A}_{\attngpusym}+T^{E}_{\expgpusym}) \cdot L = 2tnL + t \\
    P_{\sys} &= \frac{2n}{2tnL + t} 
\end{align}

The theoretical speedup is then calculated as 
\begin{align}
    \text{Speedup}_{\text{theoretical}} = \frac{P_{\sys}}{P_{EP~(Ideal)}} 
    = \frac{\frac{2n}{2tnL + t} }{\frac{3}{4Lt}} 
    &= \frac{8nL}{6nL+3}
\end{align}

Therefore, with a deep model and a large amount of micro-batches, i.e. $L$ and $n$ are big, the improvement goes up to $8/6 \approx 1.33$. Because \sys also incorporates \parallelism to realize better overlapping between communication and computation, the final speedup goes to 1.38x

But for Mixtral-W1, there are only four layers due to its larger width, the speedup is limited, and the best performance gain we achieve is xxx. This gain should further increase after 20k, however, because we only have 16GB version V100, we have to set an upper limit for \asymabbr, so the gain stop growing on 20k.
